# Supplementary material for: Learning Optimal Transport Plans Via Autoregressive Token Regression
Source: arXiv:2611.22218 source file (2026-11-17)
Supplement: Supplementary file 1 [file table_appB_runtime.tex]

\begin{table}
\caption{Time per instance (n = 30). GPU methods: single instance and batched; CPU solvers: one core.}
\label{tab:table_appB_runtime}
\begin{tabular}{lllrr}
\toprule
set & method & device & single instance [s] & batched, per instance [s] \\
\midrule
id_simplex_sqeuclidean & ToR-OT & NVIDIA A100-PCIE-40GB & 2.506 & 0.1024 \\
id_simplex_sqeuclidean & ToR-OT (transpose-averaged) & NVIDIA A100-PCIE-40GB & 5.142 & 0.2083 \\
id_simplex_sqeuclidean & Meta OT & cuda:0 & 0.0003233 & 2.61e-06 \\
id_simplex_sqeuclidean & UNOT & NVIDIA A100-PCIE-40GB & 0.008574 & 8.171e-06 \\
id_simplex_sqeuclidean & UNOT + 10 Sinkhorn steps & NVIDIA A100-PCIE-40GB & 0.008951 & 1.27e-05 \\
id_simplex_sqeuclidean & NeuralOT & GPU (several workers) & 996 & 996 \\
id_simplex_sqeuclidean & Sinkhorn GPU ε=0.01 & NVIDIA A100-PCIE-40GB & 0.02954 & 7.712e-05 \\
id_simplex_sqeuclidean & Sinkhorn GPU ε=0.001 & NVIDIA A100-PCIE-40GB & 0.2975 & 0.0008047 \\
ood_paper_sqeuclidean & ToR-OT & NVIDIA A100-PCIE-40GB & 2.493 & 0.1045 \\
ood_paper_sqeuclidean & ToR-OT (transpose-averaged) & NVIDIA A100-PCIE-40GB & 4.864 & 0.2065 \\
ood_paper_sqeuclidean & Meta OT & cuda:0 & 0.0003181 & 6.209e-06 \\
ood_paper_sqeuclidean & UNOT & NVIDIA A100-PCIE-40GB & 0.01006 & 7.011e-05 \\
ood_paper_sqeuclidean & UNOT + 10 Sinkhorn steps & NVIDIA A100-PCIE-40GB & 0.009314 & 7.885e-05 \\
ood_paper_sqeuclidean & NeuralOT & GPU (several workers) & 941.2 & 941.2 \\
ood_paper_sqeuclidean & Sinkhorn GPU ε=0.01 & NVIDIA A100-PCIE-40GB & 0.01215 & 0.0001333 \\
ood_paper_sqeuclidean & Sinkhorn GPU ε=0.001 & NVIDIA A100-PCIE-40GB & 0.1069 & 0.001259 \\
\bottomrule
\end{tabular}
\end{table}
